# Supplementary material for: Data Driven Classification of Ligand Unbinding Pathways
Source: arXiv:2308.05752 ancillary file (2023-08-02)
Supplement: Supplementary file 1 [file supp_info.pdf]

# **Supporting Information: Data Driven Classification of Ligand Unbinding Pathways**

Dhiman Ray\* and Michele Parrinello\*

*Atomistic Simulations, Italian Institute of Technology, Genoa, Via Enrico Melen 83, GE  
16153, Italy*

E-mail: [dhiman.ray@iit.it](mailto:dhiman.ray@iit.it); [michele.parrinello@iit.it](mailto:michele.parrinello@iit.it)

# Enhanced Sampling Algorithms

To accelerate the sampling of conformational transition and ligand unbinding events we used the On-the-fly Probability Enhanced Sampling (OPES),<sup>1</sup> a variant of the popular method metadynamics.<sup>2,3</sup> In OPES, a bias potential  $V(\mathbf{s})$  is constructed as a function of a collective variable (CV)  $\mathbf{s}$  that is designed to encode the slow degrees of freedom of the system. The bias potential is estimated from the instantaneous probability distribution  $P(\mathbf{s})$  constructed on-the-fly, and is given by:

$$V(\mathbf{s}) = -\frac{1}{\beta} \ln \frac{p^{\text{tg}}(\mathbf{s})}{P(\mathbf{s})}. \quad (1)$$

where  $p^{\text{tg}}(\mathbf{s})$  is the target distribution that one wishes to sample. The target distribution is usually chosen to be the well-tempered distribution  $p^{\text{tg}}(\mathbf{s}) \propto P(\mathbf{s})^{1/\gamma}$ , although other alternatives are possible. Here  $\beta$  indicates the inverse temperature and  $\gamma$  is a function of the barrier height ( $\Delta E$ ) that one wishes to overcome in the simulation. There are different variants of the OPES algorithms that are suitable for different purposes e.g. obtaining a converged free energy landscape,<sup>1,4</sup> exploration of the conformational landscape,<sup>5</sup> computing kinetics,<sup>6</sup> etc. Particularly relevant for our work are the OPES Explore<sup>5</sup> and the OPES Flooding<sup>6</sup> variants, which we use for sampling pathways and computing kinetics respectively.

## OPES Explore

The OPES Explore (OPES<sub>E</sub>) algorithm is specifically designed to quickly sample the target distribution, and thereby to increase the efficiency of conformational exploration at the expense of reduced convergence speed. Consequently, this algorithm is suitable for an initial exploration of reactive pathways in a molecular system. In OPES<sub>E</sub>, the bias potential in step  $n$  is expressed as a function of the target distribution  $p^{\text{tg}}(\mathbf{s})$  as:

$$V_n(s) = (\gamma - 1) \frac{1}{\beta} \ln \left( \frac{p_n^{\text{tg}}(s)}{Z_n} + \epsilon \right) \quad (2)$$

A regularization term  $\epsilon$  and a normalization factor  $Z$  are added to this simple expression to ensure the numerical stability of this self-consistent algorithm. The target distribution is estimated by averaging Gaussian kernels  $G_k(s, s_k)$  deposited along the CV in regular intervals:

$$p_n^{\text{tg}}(s) = \frac{1}{n} \sum_k^n G_k(s, s_k) \quad (3)$$

Molecular transition pathways explored using OPES<sub>E</sub> approach can be analyzed subsequently using DTW<sub>D</sub> to classify into different reactive channels.

## OPES Flooding

The OPES Flooding (OPES<sub>f</sub>) is designed to calculate kinetic properties from accelerated sampling by preventing bias deposition at the transition state (TS). This is achieved by ensuring the deposited bias never exceeds  $\Delta E$  which is now set to be lower than the barrier height. The bias at the iteration  $n$  is now computed as a function of the instantaneous

estimate of the marginal distribution:

$$V_n(\mathbf{s}) = (1 - 1/\gamma) \frac{1}{\beta} \log \left( \frac{P_n(\mathbf{s})}{Z_n} + \epsilon \right). \quad (4)$$

Here  $P_n(\mathbf{s})$  is the marginal probability distribution estimated at step  $n$  using weighted kernel density:

$$P_n(s) = \frac{\sum_k^n w_k G_k(s, s_k)}{\sum_k^n w_k} \quad (5)$$

where  $w_k$  is the weight of  $k$ -th kernel computed as  $w_k = \exp(\beta V_{k-1}(s_k))$ . OPES<sub>f</sub> also includes an excluded region parameter  $\chi_{\text{exc}}(s) = \mathbb{H}(s - s_{\text{exc}})$  involving a Heaviside step function  $\mathbb{H}$  that makes sure no Gaussian is deposited at  $s > s_{\text{exc}}$  to explicitly avoid biasing the TS. The unbiased kinetics of ligand unbinding  $\tau_{\text{off}}^{\text{u}}$  has been computed by rescaling the biased transition times  $\tau_{\text{off}}^{\text{b}}$  as suggested by Tiwary and Parrinello:<sup>7</sup>  $\tau_{\text{off}}^{\text{u}} = \tau_{\text{off}}^{\text{b}} \langle \exp(\beta V) \rangle_b$ , where  $V$  is the deposited bias and the ensemble average  $\langle \rangle_b$  is computed from the biased trajectory. Here, we applied OPES<sub>f</sub> algorithm in combination with DTW<sub>D</sub> to compute the kinetics of ligand unbinding along different pathways.

## Supplementary Data

### Muller Potential

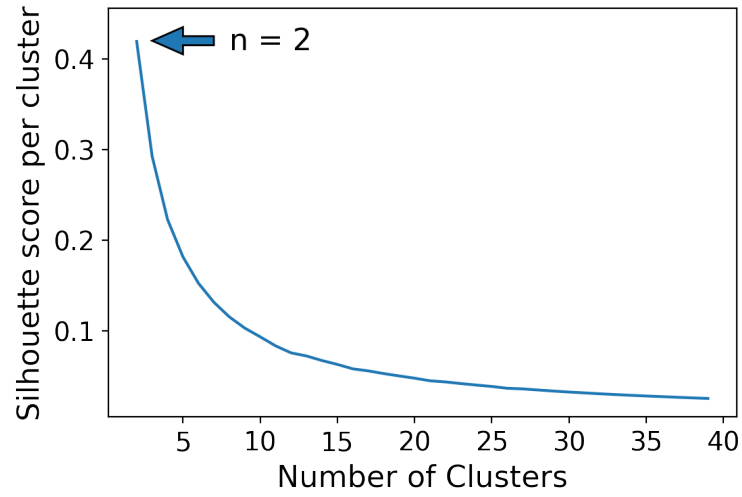

Figure S1: The results of the silhouette score test for the  $\text{DTW}_D$  clustering of the trajectories of the Muller Potential. The test indicates that the optimum number of clusters is 2.

## Alanine Dipeptide

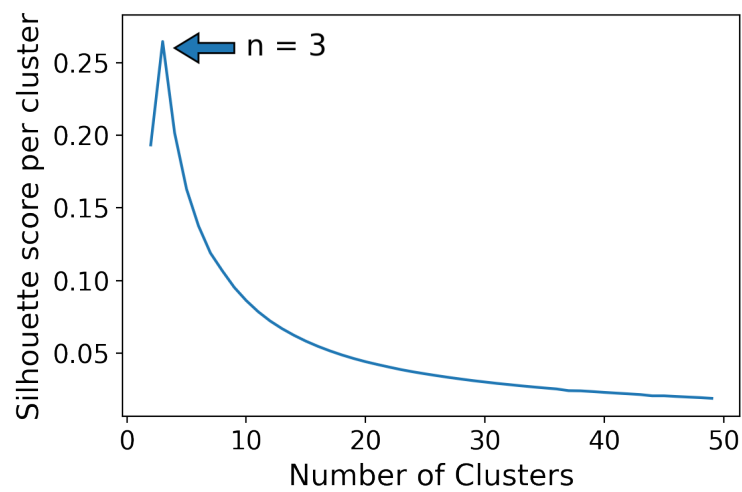

Figure S2: The results of the silhouette score test for the  $\text{DTW}_D$  clustering of the Alanine dipeptide trajectories. The test indicates that the optimum number of clusters is 3.

## Protein-Ligand complex

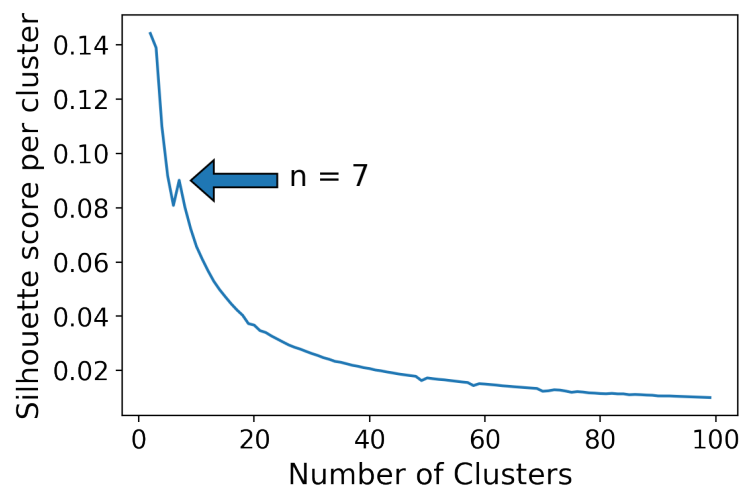

Figure S3: The results of the silhouette score test for the  $\text{DTW}_D$  clustering of the  $\text{OPES}_E$  trajectories of benzene unbinding from T4 Lysozyme. The test indicates that the optimum number of clusters is 7.

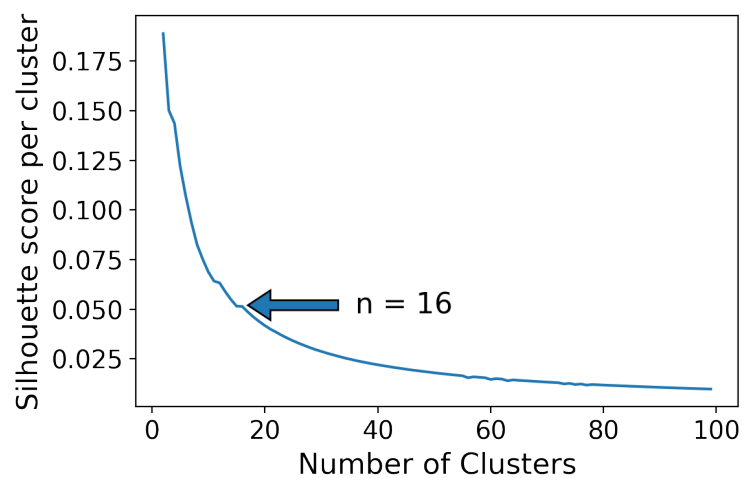

Figure S4: The results of the silhouette score test for the  $\text{DTW}_D$  clustering of the  $\text{OPES}_f$  trajectories of benzene unbinding from T4 Lysozyme. The test indicates that the optimum number of clusters is 16.

Table S1: Manual classification of 100 benzene unbinding pathways sampled from OPES<sub>E</sub> simulations.

| Path | Trajectory index                                                                                          |
|------|-----------------------------------------------------------------------------------------------------------|
| A    | 17, 20, 27, 31, 37, 51, 73, 74, 76, 89,                                                                   |
| B    | 62, 67                                                                                                    |
| C    | 5, 7, 8, 9, 10, 13, 16, 26, 30, 33, 34,<br>36, 43, 44, 45, 46, 48, 60, 61, 63, 78,<br>81, 88, 90, 91, 99, |
| D    | 3, 14, 21, 22, 24, 29, 41, 47, 50, 56,<br>57, 59, 64, 69, 70, 82, 83, 84, 85, 86,<br>96, 98, 100          |
| E    | 11, 75, 95                                                                                                |
| F    | 32, 53, 58, 71, 72, 87, 94,                                                                               |
| G    | 1, 4, 12, 15, 25, 39, 49, 55, 65, 79, 92,<br>93, 97,                                                      |
| H    | 2, 6, 18, 19, 23, 28, 35, 38, 40, 42, 52,<br>54, 66, 68, 77, 80,                                          |

Table S2: DTW<sub>D</sub> classification of 100 benzene unbinding pathways sampled from OPES<sub>E</sub> simulations.

| Medoid index | Trajectory indices                                                                                         | Path index from Manual Classification | Assigned Path index |
|--------------|------------------------------------------------------------------------------------------------------------|---------------------------------------|---------------------|
| 77           | 2, 6, 18, 19, 29, 35, 40, 42, 50, 52, 54, 66, 68, 70, 77, 84                                               | H                                     | H                   |
| 85           | 85                                                                                                         | D                                     | D2                  |
| 91           | 5, 7, 8, 9, 13, 16, 26, 30, 33, 34, 36, 43, 44, 45, 46, 48, 60, 61, 62, 63, 67, 73, 78, 81, 88, 90, 91, 99 | C                                     | C                   |
| 21           | 3, 14, 20, 21, 22, 23, 24, 41, 47, 56, 57, 59, 64, 69, 80, 82, 83, 86, 96, 98, 100                         | D                                     | D                   |
| 95           | 11, 75, 95                                                                                                 | E                                     | E                   |
| 51           | 10, 17, 27, 31, 37, 51, 74, 76, 89                                                                         | A                                     | A                   |
| 65           | 1, 4, 12, 15, 25, 28, 32, 38, 39, 49, 53, 55, 58, 65, 71, 72, 79, 87, 92, 93, 94, 97                       | F + G                                 | F + G               |

Table S3: Confusion matrix for comparing the DTW<sub>D</sub> classification with manual classification for 100 benzene unbinding pathways sampled from OPES<sub>E</sub> simulations. True positive cells are colored green. The columns indicate manually identified pathways and the rows indicate pathways clustered using DTW<sub>D</sub> algorithm. This result is also reproduced in Fig.4 in the main text.

|     | A | B | C  | D  | E | F | G  | H  |
|-----|---|---|----|----|---|---|----|----|
| A   | 8 |   | 1  |    |   |   |    |    |
| B   |   |   |    |    |   |   |    |    |
| C   | 1 | 2 | 25 |    |   |   |    |    |
| D   | 1 |   |    | 18 |   |   |    | 2  |
| D2  |   |   |    | 1  |   |   |    |    |
| E   |   |   |    |    | 3 |   |    |    |
| F+G |   |   |    |    |   | 7 | 13 | 2  |
| H   |   |   |    | 4  |   |   |    | 12 |

Table S4: The precision, recall, and F1-score for the DTW<sub>D</sub> classification of the OPES<sub>E</sub> trajectories in comparison to manual classification. The overall classification accuracy is  $\sim 96\%$  evaluated as the weighted F1-score given by:  $\sum_i N_i F_i / \sum_i N_i$ , where  $N_i$  is the number of elements in class  $i$  and  $F_i$  is the corresponding F1-score.

| Class | $N_i$ | Precision | Recall | F1 score |
|-------|-------|-----------|--------|----------|
| A     | 10    | 0.89      | 0.8    | 0.84     |
| B     | 2     | -         | 0      | -        |
| C     | 26    | 0.89      | 0.96   | 0.92     |
| D     | 23    | 0.85      | 0.78   | 0.81     |
| E     | 3     | 1.00      | 1.00   | 1        |
| F+G   | 20    | 0.91      | 1.00   | 0.95     |
| H     | 16    | 0.75      | 0.75   | 0.75     |

Table S5: Manual classification of 137 benzene unbinding pathways sampled from OPES<sub>f</sub> simulations.

| Path | Trajectory index                                                                                                                                                                                                                                                                                                                                                              |
|------|-------------------------------------------------------------------------------------------------------------------------------------------------------------------------------------------------------------------------------------------------------------------------------------------------------------------------------------------------------------------------------|
| A    | 10, 11, 15, 16, 19, 22, 34, 38, 47, 54, 58, 63, 81, 85, 86, 92, 101, 106, 111, 115, 129, 130,                                                                                                                                                                                                                                                                                 |
| B    | 12, 13, 25, 40, 43, 52, 60, 67, 87, 94, 97, 117, 119, 121, 123, 132, 137                                                                                                                                                                                                                                                                                                      |
| C    | 1, 2, 3, 4, 5, 6, 7, 8, 9, 14, 17, 18, 20, 21, 23, 28, 29, 30, 31, 32, 33, 35, 36, 37, 39, 41, 42, 44, 45, 46, 48, 49, 50, 51, 56, 57, 59, 61, 62, 64, 66, 68, 69, 70, 71, 72, 73, 74, 75, 76, 77, 78, 79, 80, 83, 84, 88, 89, 90, 91, 93, 95, 96, 98, 99, 100, 102, 103, 104, 107, 108, 109, 110, 112, 114, 118, 120, 122, 124, 125, 126, 127, 128, 131, 133, 134, 135, 136, |
| D    | 26, 27, 65,                                                                                                                                                                                                                                                                                                                                                                   |
| E    | 24, 55, 82, 105, 113,                                                                                                                                                                                                                                                                                                                                                         |
| F    | 53                                                                                                                                                                                                                                                                                                                                                                            |
| G    |                                                                                                                                                                                                                                                                                                                                                                               |
| H    | 116,                                                                                                                                                                                                                                                                                                                                                                          |

Table S6: DTW<sub>D</sub> classification of 137 benzene unbinding pathways sampled from OPES<sub>f</sub> simulations. The assignment of pathways is without the loss of any generalization as the name of the pathways are chosen arbitrarily.

| Medoid index | Trajectory index                                                                                                                                        | Path index from Manual Classification | Assigned Path index |
|--------------|---------------------------------------------------------------------------------------------------------------------------------------------------------|---------------------------------------|---------------------|
| 26           | 26, 65                                                                                                                                                  | D                                     | D1                  |
| 38           | 11, 13, 19, 38, 40, 60, 72, 101, 106, 111, 115, 129                                                                                                     | A                                     | A1                  |
| 51           | 5, 8, 17, 20, 32, 35, 39, 42, 51, 56, 62, 80, 104, 107, 109, 120, 125, 136                                                                              | C                                     | C1                  |
| 10           | 10                                                                                                                                                      | A                                     | A3                  |
| 130          | 130                                                                                                                                                     | A                                     | A4                  |
| 82           | 24, 55, 82, 105, 113                                                                                                                                    | E                                     | E                   |
| 53           | 53                                                                                                                                                      | F                                     | F                   |
| 116          | 116                                                                                                                                                     | H                                     | H                   |
| 95           | 28, 29, 33, 41, 45, 46, 61, 68, 69, 73, 74, 95, 98, 110                                                                                                 | C                                     | C2                  |
| 128          | 1, 3, 6, 21, 31, 49, 64, 71, 77, 83, 90, 99, 118, 124, 127, 128                                                                                         | C                                     | C3                  |
| 18           | 4, 18, 25, 48, 67                                                                                                                                       | C                                     | C4                  |
| 27           | 27                                                                                                                                                      | D                                     | D2                  |
| 44           | 2, 7, 9, 14, 23, 30, 36, 37, 44, 50, 57, 59, 66, 70, 75, 76, 78, 79, 84, 88, 89, 91, 93, 96, 100, 102, 103, 108, 112, 114, 122, 126, 131, 133, 134, 135 | C                                     | C5                  |
| 132          | 12, 43, 52, 94, 97, 117, 119, 121, 123, 132, 137                                                                                                        | B                                     | B1                  |
| 87           | 87                                                                                                                                                      | B                                     | B2                  |
| 15           | 15, 16, 22, 34, 47, 54, 58, 63, 81, 85, 86, 92                                                                                                          | A                                     | A2                  |

Table S7: Confusion matrix for comparing the DTW<sub>D</sub> classification with manual classification for 137 benzene unbinding pathways sampled from OPES<sub>f</sub> simulations. True positive cells are colored green. The columns indicate manually identified pathways and the rows indicate pathways clustered using DTW<sub>D</sub> algorithm. When multiple clusters are identified within one unbinding pathway, all such clusters are considered true positive. The only exception is when a cluster has only one trajectory but there are multiple transitions sampled for that pathway. It is not possible to determine whether such a cluster is true positive or false positive as each cluster is associated with a pathway through visual inspection. So such cells are marked yellow and are excluded from the calculation of classification accuracy.

|    | A  | B  | C  | D | E | F | H |
|----|----|----|----|---|---|---|---|
| A1 | 9  | 3  |    |   |   |   |   |
| A2 | 12 |    |    |   |   |   |   |
| A3 | 1  |    |    |   |   |   |   |
| A4 | 1  |    |    |   |   |   |   |
| B1 |    | 11 |    |   |   |   |   |
| B2 |    | 1  |    |   |   |   |   |
| C1 |    |    | 18 |   |   |   |   |
| C2 |    |    | 14 |   |   |   |   |
| C3 |    |    | 16 |   |   |   |   |
| C4 |    | 2  | 3  |   |   |   |   |
| C5 |    |    | 36 |   |   |   |   |
| D1 |    |    |    | 2 |   |   |   |
| D2 |    |    |    | 1 |   |   |   |
| E  |    |    |    |   | 5 |   |   |
| F  |    |    |    |   |   | 1 |   |
| H  |    |    |    |   |   |   | 1 |

Table S8: The precision, recall, and F1-score for the DTW<sub>D</sub> classification of the OPES<sub>f</sub> trajectories in comparison to manual classification. The overall classification accuracy is  $\sim 96\%$  evaluated as the weighted F1-score given by:  $\sum_i N_i F_i / \sum_i N_i$ , where  $N_i$  is the number of elements in class  $i$  and  $F_i$  is the corresponding F1-score.

| Class | $N_i$ | Precision | Recall | F1-score |
|-------|-------|-----------|--------|----------|
| A     | 21    | 0.875     | 1.00   | 0.93     |
| B     | 16    | 1.0       | 0.69   | 0.82     |
| C     | 87    | 0.98      | 1.0    | 0.99     |
| D     | 2     | 1.0       | 1.0    | 1.00     |
| E     | 5     | 1.0       | 1.0    | 1.00     |
| F     | 1     | 1.0       | 1.0    | 1.00     |
| H     | 1     | 1.0       | 1.0    | 1.00     |

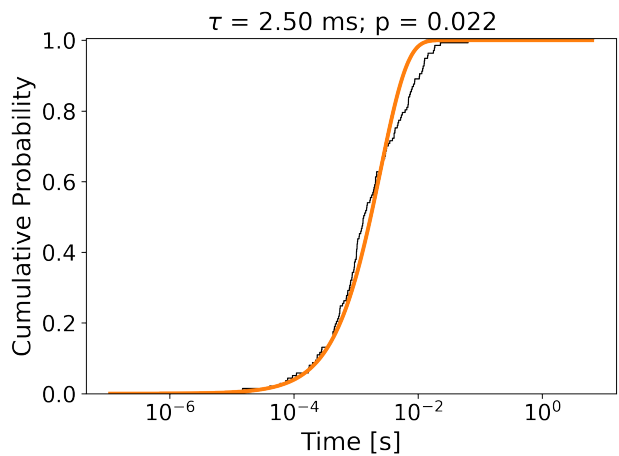

Figure S5: The cumulative distribution of the timescales of benzene unbinding from T4 Lysozyme computed from OPES<sub>f</sub> simulations. This plot includes the results of all 137 unbinding transitions along different pathways taken together. The  $p$ -value of the Kolmogorov-Smirnov (KS) test is less than 0.05. It indicates that these datasets do not follow a single exponential distribution, which makes the estimated residence time statistically unreliable. Nevertheless, the single exponential fit of the entire dataset is shown in orange.

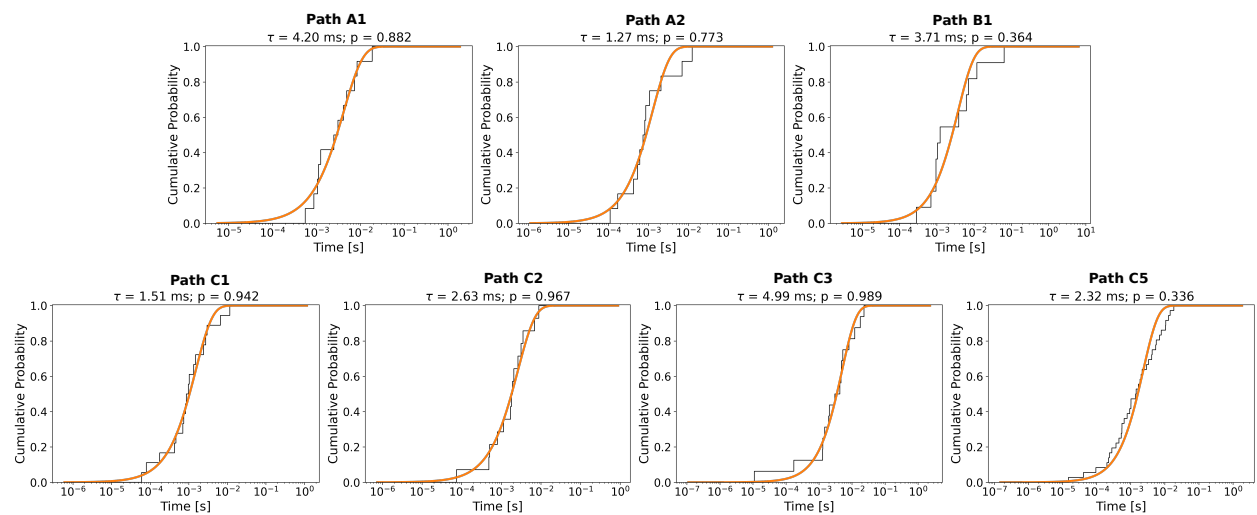

Figure S6: The cumulative distribution of the benzene unbinding timescales along different path clusters identified through DTW<sub>D</sub> algorithm. Results are shown only for those clusters where  $\geq 10$  unbinding transitions were observed. The  $p$ -value of the Kolmogorov-Smirnov (KS) test is much more than 0.05. It indicates that each of these datasets follows a single exponential distribution on its own.

## Role of Protein residues in distinguishing ligand release paths with different timescales.

To understand the role of protein residues in affecting the kinetics within a single pathway, we performed one-dimensional dynamic time warping on the time series of each descriptor, to

measure the cumulative distance between different clusters belonging to one pathway. This analysis identified the role of individual protein residues in determining the unbinding kinetics (Fig. S7). For example, Lys83 and Arg119 distinguish between the two clusters within Pathway A, determining whether the unbinding time is  $\sim 1.3$  ms or  $\sim 4.2$  ms. Moreover, Ile3, Asn68, and Ala97 residues determine which subclass of unbinding pathways is followed within Path C leading to a difference in the dissociation timescale.

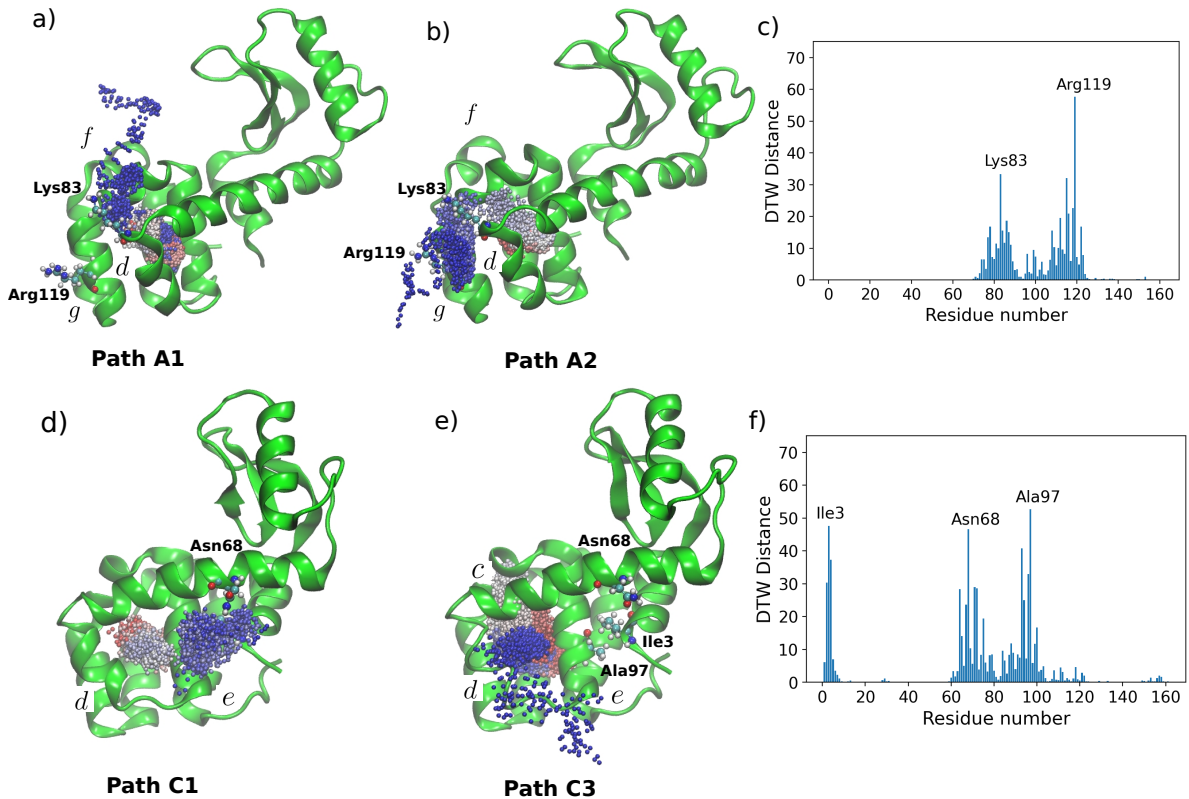

Figure S7: The different protein residues that distinguish the different ligand unbinding channels within a visually distinguishable pathway. Panel (a) and (b) show two such channels within Path A. These two channels are separated by the interaction of the ligand with the Lys83 and Arg119 residues. The two residues are explicitly shown in (a) and (b). Panel (c) shows the DTW distance between these two channels for each protein residue. It is indicative that the ligand coordination with Lys83 and Arg119 residues best discriminates the two dissociation channels. Panel (d),(e), and (f) are identical to (a),(b), and (c) respectively except that it demonstrates the distinction between two dissociation channels within Path C.

## References

- (1) Invernizzi, M.; Piaggi, P. M.; Parrinello, M. Unified Approach to Enhanced Sampling. *Physical Review X* **2020**, *10*, 041034.
- (2) Laio, A.; Parrinello, M. Escaping free-energy minima. *Proceedings of the National Academy of Sciences of the United States of America* **2002**, *99*, 12562–6.
- (3) Barducci, A.; Bussi, G.; Parrinello, M. Well-Tempered Metadynamics: A Smoothly Converging and Tunable Free-Energy Method. *Physical Review Letters* **2008**, *100*, 020603.
- (4) Invernizzi, M.; Parrinello, M. Rethinking Metadynamics: From Bias Potentials to Probability Distributions. *Journal of Physical Chemistry Letters* **2020**, *11*, 2731–2736.
- (5) Invernizzi, M.; Parrinello, M. Exploration vs Convergence Speed in Adaptive-Bias Enhanced Sampling. *Journal of Chemical Theory and Computation* **2022**, *18*, 3988–3996.
- (6) Ray, D.; Ansari, N.; Rizzi, V.; Invernizzi, M.; Parrinello, M. Rare Event Kinetics from Adaptive Bias Enhanced Sampling. *Journal of Chemical Theory and Computation* **2022**, *18*, 6500–6509.
- (7) Tiwary, P.; Parrinello, M. From metadynamics to dynamics. *Physical review letters* **2013**, *111*, 230602.
